# Supplementary material for: Learning Interpretable Policies in Hindsight-Observable POMDPs through Partially Supervised Reinforcement Learning
Source: arXiv:2402.09290 source file (2024-02-14)
Supplement: Supplementary file 1 [file appendix.tex]

subsection{State Representation in POMDPs}
\label{state_representation}

In a POMDP, an agent doesn't observe the real state \( s_t \) but instead gets an observation \( o_t \) that is correlated with the real state. The history window \( h_t \) is often used as a surrogate state:
\begin{equation}
h_t = \{o_{t-k+1}, \dots, o_t\}
\end{equation}
where \( k \) determines the size of the observation window. 

The inherent limitation here is the state's Markov property. Even with history windows, many real-world scenarios may not render the surrogate state \( h_t \) Markovian, leading to suboptimal policies. Formally, a state \( s \) is Markovian if:
\begin{equation}
P(s_{t+1}|s_t, a_t) = P(s_{t+1}|s_0, a_0, \dots, s_t, a_t)
\end{equation}
For a surrogate state \( h_t \) to be Markovian, the history window needs to capture all relevant information about past states and actions, which may not always be feasible or efficient with increasing \( k \).

It is plausible to posit that we can approximate the solution of a POMDP by considering it as an MDP under certain conditions.
Consider the following assumptions:

\begin{assumption}
For every true state $s_t$ there exists a learned state estimation $\hat{s}_t$ such that $\forall\epsilon>0$:
\begin{equation}
||\hat{s}_t - s_t|| \leq \epsilon
\end{equation}
\end{assumption}

\begin{assumption}
For any state \( s \), action \( a \), and any other latent factors \( z \), the probabilistic transition function \( T \) and the reward model \( R \) satisfy:
\begin{align*}
T(s, a, z) &\approx T(s, a) \\
R(s, a, z) &\approx R(s, a)
\end{align*}
indicating that the influence of \( z \) on the transition dynamics and resulting reward is minimal compared to the influence of state \( s \).
\end{assumption}

In a POMDP, the observation function \( O \) is traditionally responsible for mapping states \( s \) to observations \( o \). Specifically, the probability of observing \( o_t \) given that the real state is \( s_t \) is denoted as \( O(o_t|s_t) \). 

Given Assumption 3.1, as \( \hat{s}_t \) converges to \( s_t \), the observation function starts to resemble an identity mapping from the state space \( S \) to itself. That is:
\[ \lim_{\hat{s}_t \to s_t} O(\hat{s}_t|s_t) = 1 \]
And for any \( \hat{s}_t \neq s_t \):
\[ \lim_{\hat{s}_t \to s_t} O(\hat{s}_t|s_t) = 0 \]

This effectively transforms the POMDP into an MDP as the observations converge to state. This is of theoretical importance because, under this scenario, we can use Bellman's equation to bound the rewards of policies generated with estimated states.

Given this, and the previous assumption regarding the closeness of \( \hat{s} \) to \( s \), it can be deduced that the Q-value for a policy using the true state serves as an upper bound for that using the approximated state:
\begin{theorem}
For a policy \(\pi\), given the assumptions on state representation and environmental dynamics, as the estimated state \(\hat{s}\) converges to the true state \(s\), the corresponding Q-value for the estimated state converges to the Q-value for the true state:
\[ \lim_{\hat{s} \to s} \hat{Q}^*(\hat{s}, a) = Q^*(s, a) \]
\end{theorem}

\begin{proof}
Starting from the Bellman optimality equations, we have:
\[ Q^*(s, a) = \mathbb{E}[R(s, a) + \gamma \max_{a'} Q^*(T(s, a), a')] \]
\[ \hat{Q}^*(\hat{s}, a) = \mathbb{E}[R(\hat{s}, a) + \gamma \max_{a'} \hat{Q}^*(T(\hat{s}, a), a')] \]

Given Assumption 3.1, as \( \hat{s}_t \) converges to \( s_t \), the policy decision based on \(\hat{s}_t\) converges to the decision based on \(s_t\).

From Assumption 3.2, as \( \hat{s} \rightarrow s \), the influence of latent variables \( z \) on the transition dynamics and reward function diminishes. Formally:
\[ \lim_{\hat{s} \to s} T(s, a, z) = T(s, a) \]
\[ \lim_{\hat{s} \to s} R(s, a, z) = R(s, a) \]

Substituting these converging relations into the Bellman equations and taking the limit as \( \hat{s} \rightarrow s \) yields:
\[ \lim_{\hat{s} \to s} \hat{Q}^*(\hat{s}, a) = \mathbb{E}[R(s, a) + \gamma \max_{a'} Q^*(T(s, a), a')] \]

Which is precisely the Bellman equation for \( Q^*(s, a) \). Thus, it can be concluded that:
\[ \lim_{\hat{s} \to s} \hat{Q}^*(\hat{s}, a) = Q^*(s, a) \]
\end{proof}
\begin{theorem}
Given an optimal policy \(\pi^*\), the expected reward using the true state serves as an upper bound on the expected reward using the approximated state, i.e.,
\[ V^*(s) \geq \hat{V}^*(\hat{s}) \]
for all \( s \) and corresponding \( \hat{s} \).
\end{theorem}

\begin{proof}
For any state \( s \) and action \( a \), the Bellman optimality equation can be expressed as:
\[ V^*(s) = \max_a \mathbb{E}[R(s, a) + \gamma V^*(T(s, a))] \]
\[ \hat{V}^*(\hat{s}) = \max_a \mathbb{E}[R(\hat{s}, a) + \gamma \hat{V}^*(T(\hat{s}, a))] \]

From our previously established result, we know that:
\[ \lim_{\hat{s} \to s} \hat{Q}^*(\hat{s}, a) = Q^*(s, a) \]
Given that the Q-function essentially captures the expected reward of taking action \( a \) in state \( s \) (or \( \hat{s} \)), the expected reward from the true state is at least as much as that from the estimated state, thus:
\[ Q^*(s, a) \geq \hat{Q}^*(\hat{s}, a) \]
for all \( s \), \( \hat{s} \), and \( a \).

Given that the value function is a maximization over Q-values for all actions, we can deduce that:
\[ V^*(s) = \max_a Q^*(s, a) \geq \max_a \hat{Q}^*(\hat{s}, a) = \hat{V}^*(\hat{s}) \]

Thus, the expected cumulative reward from the true state using the optimal policy is always greater than or equal to that from the approximated state.
\end{proof}

This holds in particular for \( V(s_{\text{terminal}}) \) which is defined as the reward over the policy given its state history. It therefore follows that the reward of a policy using true states serves as an upper bound to the reward of a policy using state estimations under assumptions 3.1 and 3.2.

So far we have been using the term "state estimation" without explaining how it is obtained. Next we will present our methods to obtaining this.
